# Supplementary material for: Fast calculation of two-electron-repulsion integrals: a numerical approach
Source: arXiv:1609.06633 source file (2016-09-21)
Supplement: Supplementary file 1 [file SuppMatt.pdf]

# Supplemental Material

Fast calculation of two-electron-repulsion integrals: a numerical approach

*Pedro E. M. Lopes*

*Rua Almirante Reis, Nº 28A, 2º Esq, 2330-099 Entroncamento, Portugal*

mail: plopesuk@yahoo.co.uk

Website: www.fastcompchem.com

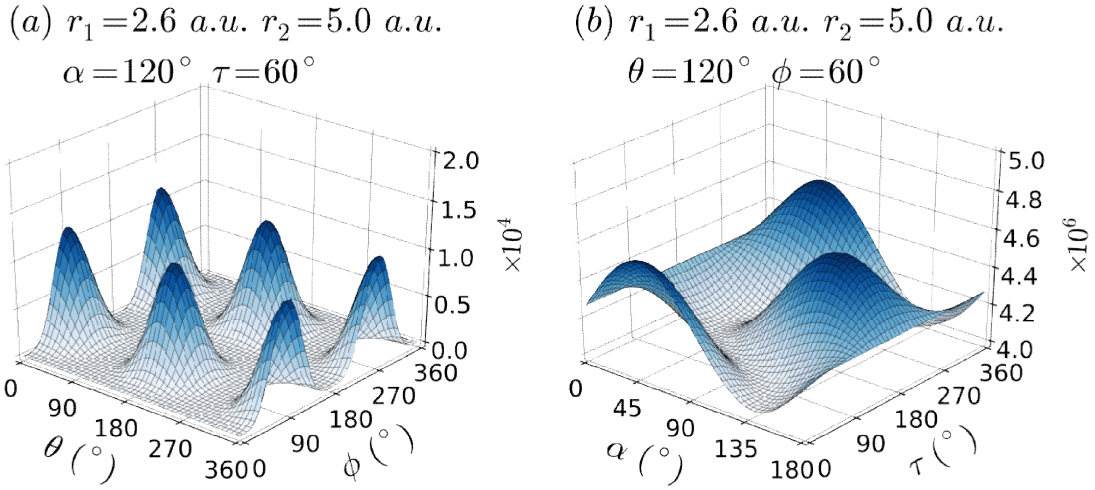


**Figure S1** Symmetry properties of the surfaces (θ, φ) and (α, τ) of $g_4^{rot}(\overline{PQ}_x^4)$. In (a) α = 120º and τ = 60º and in (b) θ = 120º and φ = 60º. For both (a) and (b) $r_1$ = 2.6 a.u. and $r_2$ = 5.0 a.u.

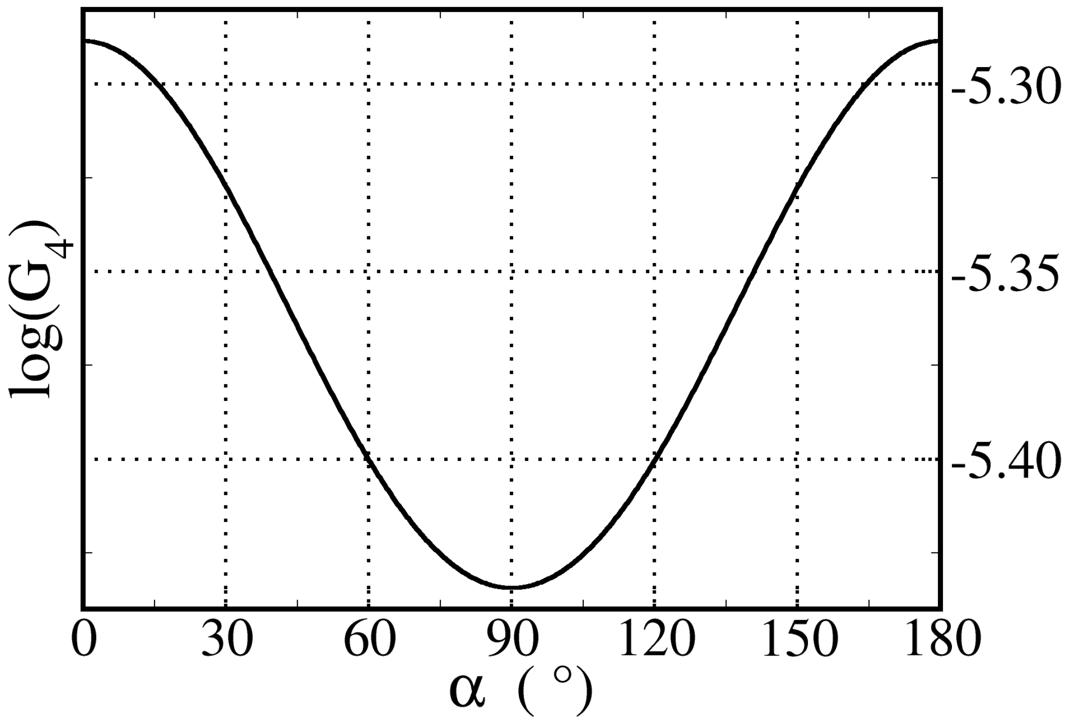


**Figure S2** Plot of $G_4(\alpha)$ for $r_1$ = 2.6 a.u. and $r_2$ = 5.0 a.u. The curve is symmetric at α = 90º and was approximated by a tenth-order polynomial.

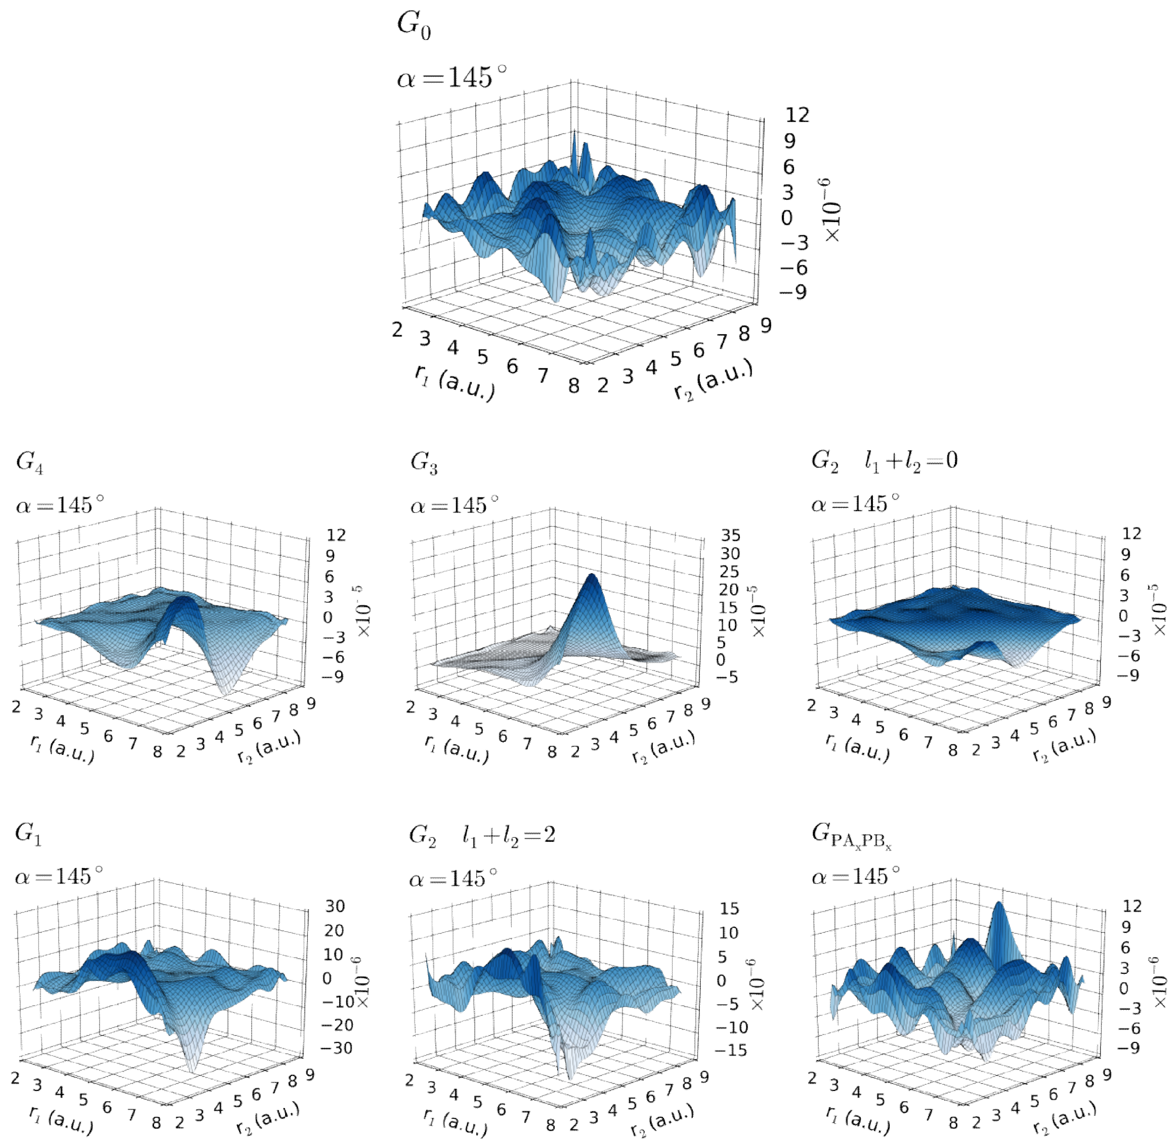


**Figure S3** Illustration of the residuals of $G_n(r_1, r_2)$ and $G_{\overline{PA}_x\overline{PB}_x}(r_1, r_2)$ for α=145°. The term $G_0$ is highlighted since it makes a direct contribution to the computed ERI.
